# Supplementary material for: Periodic implementation of the random phase approximation with numerical atomic orbitals and dual reciprocal space grids
Source: arXiv:2505.06021 ancillary file (2025-08-29)
Supplement: Supplementary file 1 [file SI_RPA_paper.pdf]

# Supporting Information to "Periodic implementation of the random phase approximation with numerical atomic orbitals and dual reciprocal space grids"

Edoardo Spadetto,[*,†,‡] Pier Herman Theodoor Philipsen,[*,‡] Arno Förster,[*,†] and Lucas Visscher[*,†]

†*Theoretical Chemistry, Vrije Universiteit, De Boelelaan 1108, 1081 HZ Amsterdam, The Netherlands*

‡*Software for Chemistry and Materials NV, NL, 1081HV, Amsterdam, The Netherlands*

E-mail: e.spadetto@vu.nl; philipsen@scm.com; a.t.l.foerster@vu.nl; l.visscher@vu.nl

## Contents

**S1 Comparison between molecules and periodic system** **2**

S1.1 Results: Noble gas chains . . . . . . . . . . . . . . . . . . . . . . . . . 3

**S2 3D simple cubic Noble Gases topologies** **4**

**S3 MgO-CO** **7**

S3.1 SCF Energies . . . . . . . . . . . . . . . . . . . . . . . . . . . . . . . . 8

S3.2 Absolute RPA Correlation energies . . . . . . . . . . . . . . . . . . . . 9

**References** **9**

# S1 Comparison between molecules and periodic system

Consider a 1D system with lattice constant $a$ and basis set $\{\chi_\mu(k_i)\}$. The basis functions are

$$\chi_\mu(\boldsymbol{r}, k_i) = \sum_n e^{ik_i \cdot na} \chi_\mu(\boldsymbol{r} - na) \tag{1}$$

Splitting the Bloch sum to consider the distance between two primitive cells we get

$$\begin{aligned}
\chi_\mu(\boldsymbol{r}, k_i) &= \sum_n e^{ik_i 2na} \chi_\mu(\boldsymbol{r} - 2na) + e^{ik_i(2n+1)a} \chi_\mu(\boldsymbol{r} - (2n+1)a) & (2)\\
&= \sum_n e^{ik_i n(2a)} \chi_{\mu'}(\boldsymbol{r} - 2an) + e^{ik_i a} e^{ik_i n(2a)} \chi_{\mu''}(\boldsymbol{r} - 2an) & (3)\\
&= \chi_{\mu'}(\boldsymbol{r}, k_i) + e^{ik_i a} \chi_{\mu''}(\boldsymbol{r}, k_i) & (4)
\end{aligned}$$

Where the indices $\mu'$ and $\mu''$ and removal of the translation factor $a$, comes from substituting with basis functions from the system with two supercells.

This proves that every Bloch's sum basis function of the single primitive cell can be rewritten with the basis set from the system with a doubled primitive cell. The inverse however is not true, because in principle the 2 supercell system can break translational symmetry within the two unit cells. The case of a single unit cell is more restrictive because the next unit cell is forced to respect translational invariance as an ansatz. Nevertheless, even though a larger Hilbert space can be represented with the two supercell case, the translational invariance of one single cell should be respected by any physical solution..

Going from the single to the double unit cell case, the size of the first Brillouin zone of

the system halves,

$$
\begin{aligned}
\chi_\mu(k_i = k_j + \frac{\pi}{a}) &= \chi_{\mu'}(\boldsymbol{r}, k_i) + e^{ik_i a}\chi_{\mu''}(\boldsymbol{r}, k_i) \qquad (5) \\
&= \sum_n \left(e^{ik_i 2na}\chi_{\mu'}(\boldsymbol{r} - 2an) + e^{ik_i a}e^{ik_i 2na}\chi_{\mu''}(\boldsymbol{r} - 2an)\right) \\
&= \sum_n \left(e^{i(k_j+\frac{\pi}{a})2na}\chi_{\mu'}(\boldsymbol{r} - 2an) + e^{i(k_j+\frac{\pi}{a})a}e^{i(k_j+\frac{\pi}{a}))2na}\chi_{\mu''}(\boldsymbol{r} - 2an)\right) \\
&= e^{2\pi i}\sum_n \left(e^{ik_j 2na}\chi_{\mu'}(\boldsymbol{r} - 2an) + e^{i(k_j+\frac{\pi}{a})a}e^{ik_j 2na}\chi_{\mu''}(\boldsymbol{r} - 2an)\right) \\
&= \sum_n \left(e^{ik_j 2na}\chi_{\mu'}(\boldsymbol{r} - 2an) - e^{ik_j a}e^{ik_j 2na}\chi_{\mu''}(\boldsymbol{r} - 2an)\right) \\
&= \chi_{\mu'}(\boldsymbol{r}, k_j) - e^{ik_j a}\chi_{\mu''}(\boldsymbol{r}, k_j) \ .
\end{aligned}
$$

This equation shows that if we consider any basis function at a certain $\boldsymbol{k}$ point in the first Brillouin zone, from the single unit cell system we can rewrite it using functions from the double cell case, with the same, or with a $\boldsymbol{k}$-coordinate translated by half of the first Brillouin zone. This means, that now the Brillouin zone has dimension $\pi/a$ and not as the 1 supercell case $2\pi/a$. Together, these two arguments are valid for an arbitrary number of considered primitive cells. This proves that as a limit, even an infinite-size molecule consisting of an infinite number of primitive cells evaluated only at the Γ-point, will give the same results as a periodic calculation with a converged $\boldsymbol{k}$-grid and a single unit cell.

Clearly, this infinite molecule calculation cannot be evaluated. In practice, we extrapolate RPA correlation energy for molecules of increasing size to the infinite length limit, with the assumption that the effects coming from the different boundary conditions would be local.

## S1.1 Results: Noble gas chains

To prove the correctness of this periodic code we compared it with a molecular implementation[1] for noble gas chains. The boundary effects are removed from the molecular calculation

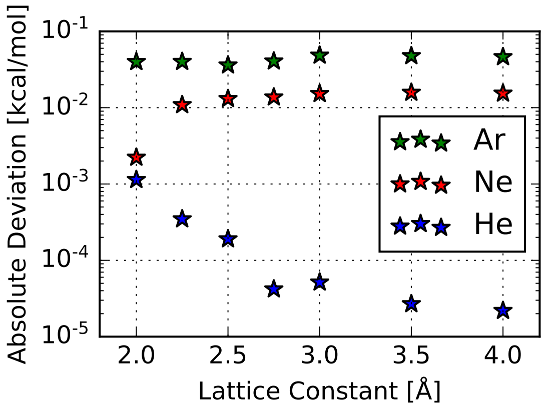


Figure S1: Absolute deviation between extrapolated molecular RPA correlation energy per atom for an infinite chain of noble gas atoms, compared with periodic result.

by fitting the total RPA Correlation linearly for multiple lengths with

$$E_{corr}^{RPA}(N) = aN + b \tag{6}$$

this way the parameter $a$ contains the correlation energy per unit cell without boundary effects. Instead, the periodic calculation is converged directly using a regular $K_G/Q_G$ of 40 $\boldsymbol{k}$-points. Calculations are performed with the `STO/TZ2P` basis set.

# S2 3D simple cubic Noble Gases topologies

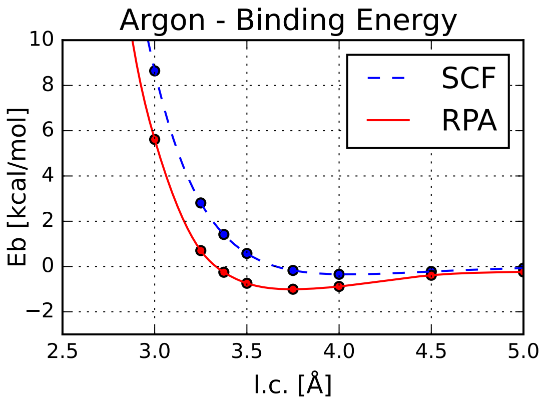


Figure S2: RPA@PBE binding energy of Argon in a simple cubic lattice structure.

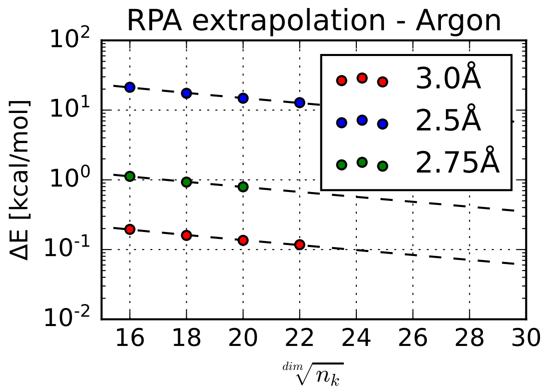


Figure S3: Extrapolation of RPA@PBE binding energies of Argon in a simple cubic lattice structure to the infinite $\boldsymbol{k}$-grid limit for different lattice constants.

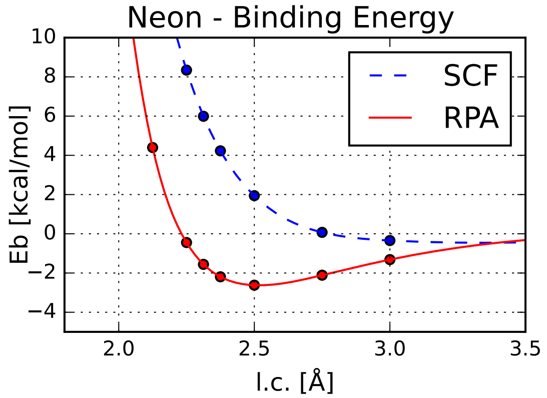


Figure S4: RPA@PBE binding energy of Neon in a simple cubic lattice structure.

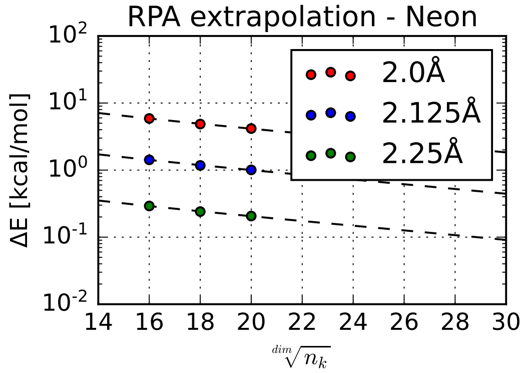


Figure S5: Extrapolation of RPA@PBE binding energies of Neon in a simple cubic lattice structure to the infinite $\boldsymbol{k}$-grid limit for different lattice constants.

Table S1: Equilibrium lattice constants for simple cubic Neon and Argon crystals with TZ2P basis set

| | SCF [Å] | RPA[Å] |
|---|---|---|
| Ne | 3.34 | 2.43 |
| Ar | 4.06 | 3.74 |

As done by Kresse and coworkers for FCC crystals,[2] we here calculated RPA@PBE binding energy curves of noble gas simple cubic lattices, highlighting how adopting the RPA correction describes the stability valley prescribed by van der Waals theory. The calculations involving Argon and Neon crystals can be seen in S2 and S4 respectively. For the tightest lattice constants $E_{corr}^{RPA}$ has been extrapolated through a $a\frac{1}{\sqrt[dim]{n_k}} + b$ fit.[3] For the larger lattice constants, no extrapolation was required to obtain converged results. Details about the correctness of the extrapolation can be seen in figures S3 and S5, where we report the absolute deviation of the RPA correlation energies with respect to the extrapolated value for a few lattice constants. The detailed prospect of extrapolated and non-extrapolated lattice constants can be found in tables S2, S3. Table S1 shows the equilibrium lattice constants which are obtained as the minima of the binding energy curves shown in Figs. S2 and S4.

Table S2: RPA@PBE binding energies of Argon in a simple cubic lattice. The table shows whether a lattice constant has been extrapolated to the infinite $\boldsymbol{k}$-point limit, the lattice constant, the number of points in the regular $K_G/Q_G$ per dimension, the number of frequencies used, and the energy deviation of the extrapolated results with respect to the one obtained with the highest accuracy.

| Extrapolated | l.c. | $\sqrt[ndim]{n_k}$ | $n_\omega$ | $\Delta E$ |
|---|---|---|---|---|
| True | 2.5 | [16, 18, 20, 22] | 32 | 22.71 |
| True | 2.75 | [16, 18, 20] | 32 | 1.31 |
| True | 3.0 | [16, 18, 20, 22] | 32 | 0.20 |
| False | 3.25 | [16, 18] | 32 | 0.0 |
| False | 3.375 | [16, 18] | 32 | 0.0 |
| False | 3.5 | [16, 18] | 32 | 0.0 |
| False | 3.75 | [16] | 32 | 0.0 |
| False | 4.0 | [18] | 32 | 0.0 |
| False | 4.5 | [14] | 32 | 0.0 |
| False | 5.0 | [16] | 32 | 0.0 |
| False | 5.5 | [14] | 32 | 0.0 |
| False | 8.0 | [14] | 32 | 0.0 |

Table S3: RPA@PBE binding energies of Neon in a simple cubic lattice. The table shows whether a lattice constant has been extrapolated to the infinite $\boldsymbol{k}$-point limit, the lattice constant, the number of points in the regular $K_G/Q_G$ per dimension, the number of frequencies used, and the energy deviation of the extrapolated results with respect to the one obtained with the highest accuracy.

| Extrapolated | l.c. | $\sqrt[ndim]{n_k}$ | $n_\omega$ | $\Delta E$ |
|---|---|---|---|---|
| True | 1.5 | [16, 18, 20] | 32 | 1298.16 |
| True | 2.0 | [16, 18, 20] | 32 | 6.92 |
| True | 2.125 | [16, 18, 20] | 32 | 1.67 |
| True | 2.25 | [16, 18, 20] | 32 | 0.34 |
| True | 2.3125 | [16, 18, 20] | 32 | 0.18 |
| True | 2.375 | [16, 18, 20] | 32 | 0.11 |
| True | 2.5 | [16, 18, 20] | 32 | 0.073 |
| True | 2.75 | [16, 18, 20] | 32 | 0.0423 |
| True | 3.0 | [16, 18, 20] | 32 | 0.0277 |
| True | 3.5 | [8, 10, 12, 14] | 32 | 0.02406 |
| False | 4.0 | [18] | 32 | 0.0 |
| False | 4.5 | [14] | 32 | 0.0 |
| False | 5.0 | [18] | 32 | 0.0 |
| False | 5.5 | [14] | 32 | 0.0 |
| False | 10.0 | [20] | 32 | 0.0 |

# S3 MgO-CO

Here we report details of the results obtained for MgO-CO the adsorption for different basis sets, functionals, and coverage.

## S3.1 SCF Energies

Table S4: Energy terms from SCF PBE Calculation in Hartree.

| | CO + MgO | MgO | CO |
|---|---|---|---|
| DZP 100% 4l | | | |
| PBE | −2.230 245 | −1.693 543 | −0.531 876 |
| HFX@PBE | −120.414 515 | −105.718 950 | −14.690 824 |
| XC@PBE | −2.448 933 | −2.011 719 | −0.415 042 |
| TZ2P 100% 4l | | | |
| PBE | −2.257 428 | −1.711 354 | −0.540 658 |
| HFX@PBE | −120.417 549 | −105.709 182 | −14.703 534 |
| XC@PBE | −2.446 996 | −1.998 771 | −0.427 299 |
| QZ4P 100% 4l | | | |
| PBE | −2.259 670 | −1.712 464 | −0.541 637 |
| XC@PBE | −2.447 122 | −1.999 157 | −0.426 992 |
| TZ2P 50% 2l | | | |
| PBE | −2.228 480 | −1.676 423 | −0.547 291 |
| HFX@PBE | −110.734 627 | −97.440 143 | −13.285 696 |
| XC@PBE | −2.320 930 | −1.888 212 | −0.407 755 |
| TZ2P 25% 2l | | | |
| PBE | −3.905 066 | −3.352 806 | −0.547 199 |
| HFX@PBE | −208.173 398 | −194.878 634 | −13.285 750 |
| XC@PBE | −4.208 540 | −3.776 461 | −0.407 232 |
| TZ2P 100% 3l | | | |
| PBE | −1.820 828 | −1.274 841 | −0.540 657 |
| HFX@PBE | −93.960 486 | −79.252 670 | −14.703 519 |
| XC@PBE | −1.919 010 | −1.471 344 | −0.427 297 |

## S3.2 Absolute RPA Correlation energies

Table S5: RPA Correlation energy @ PBE, different coverages, different number of layers

| $\sqrt[dim]{n_k}$ | CO + MgO | CO | MgO |
|---|---|---|---|
| DZP 100% 4l | | | |
| 11 | −2.276 887 | −0.503 965 | −2.791 350 |
| 9 | −2.276 630 | −0.503 948 | −2.791 110 |
| 13 | −2.277 049 | −0.503 968 | −2.791 505 |
| TZ2P 100% 4l | | | |
| 11 | −2.677 042 | −0.595 905 | −3.285 316 |
| 9 | −2.676 603 | −0.595 936 | −3.284 952 |
| 13 | −2.677 127 | −0.595 971 | −3.285 458 |
| TZ2P 100% 3l | | | |
| 11 | −2.005 798 | −0.596 022 | −2.614 233 |
| 9 | −2.009 201 | −0.596 280 | −2.617 905 |
| 13 | −2.005 923 | −0.596 055 | −2.614 381 |
| TZ2P 50% 2l | | | |
| 9 | −2.683 181 | −0.589 478 | −3.283 942 |
| 11 | −2.683 309 | −0.589 487 | −3.284 079 |
| 13 | −2.683 425 | −0.589 490 | −3.284 194 |
| TZ2P 25% 2l | | | |
| 5 | −5.367 212 | −0.587 849 | −5.966 110 |
| 7 | −5.368 292 | −0.587 910 | −5.967 264 |

# References


(1) Spadetto, E.; Philipsen, P. H. T.; Förster, A.; Visscher, L. Toward Pair Atomic Density Fitting for Correlation Energies with Benchmark Accuracy. *J. Chem. Theory Comput.* **2023**, *19*, 1499–1516.

(2) Harl, J.; Kresse, G. Cohesive energy curves for noble gas solids calculated by adiabatic connection fluctuation-dissipation theory. *Phys. Rev. B* **2008**, *77*, 045136.

(3) Ren, X.; Merz, F.; Jiang, H.; Yao, Y.; Rampp, M.; Lederer, H.; Blum, V.; Scheffler, M. All-electron periodic G0W0 implementation with numerical atomic orbital basis functions: Algorithm and benchmarks. *Phys. Rev. Mater.* **2021**, *5*, 013807.
